# Supplementary material for: Marginalized Beam Search Algorithms for Hierarchical HMMs
Source: arXiv:2305.11752 source file (2023-05-19)
Supplement: Supplementary file 1 [file appendix_x.tex]

\begin{figure}[!htp]
  \centering
  \includegraphics[scale=0.45]{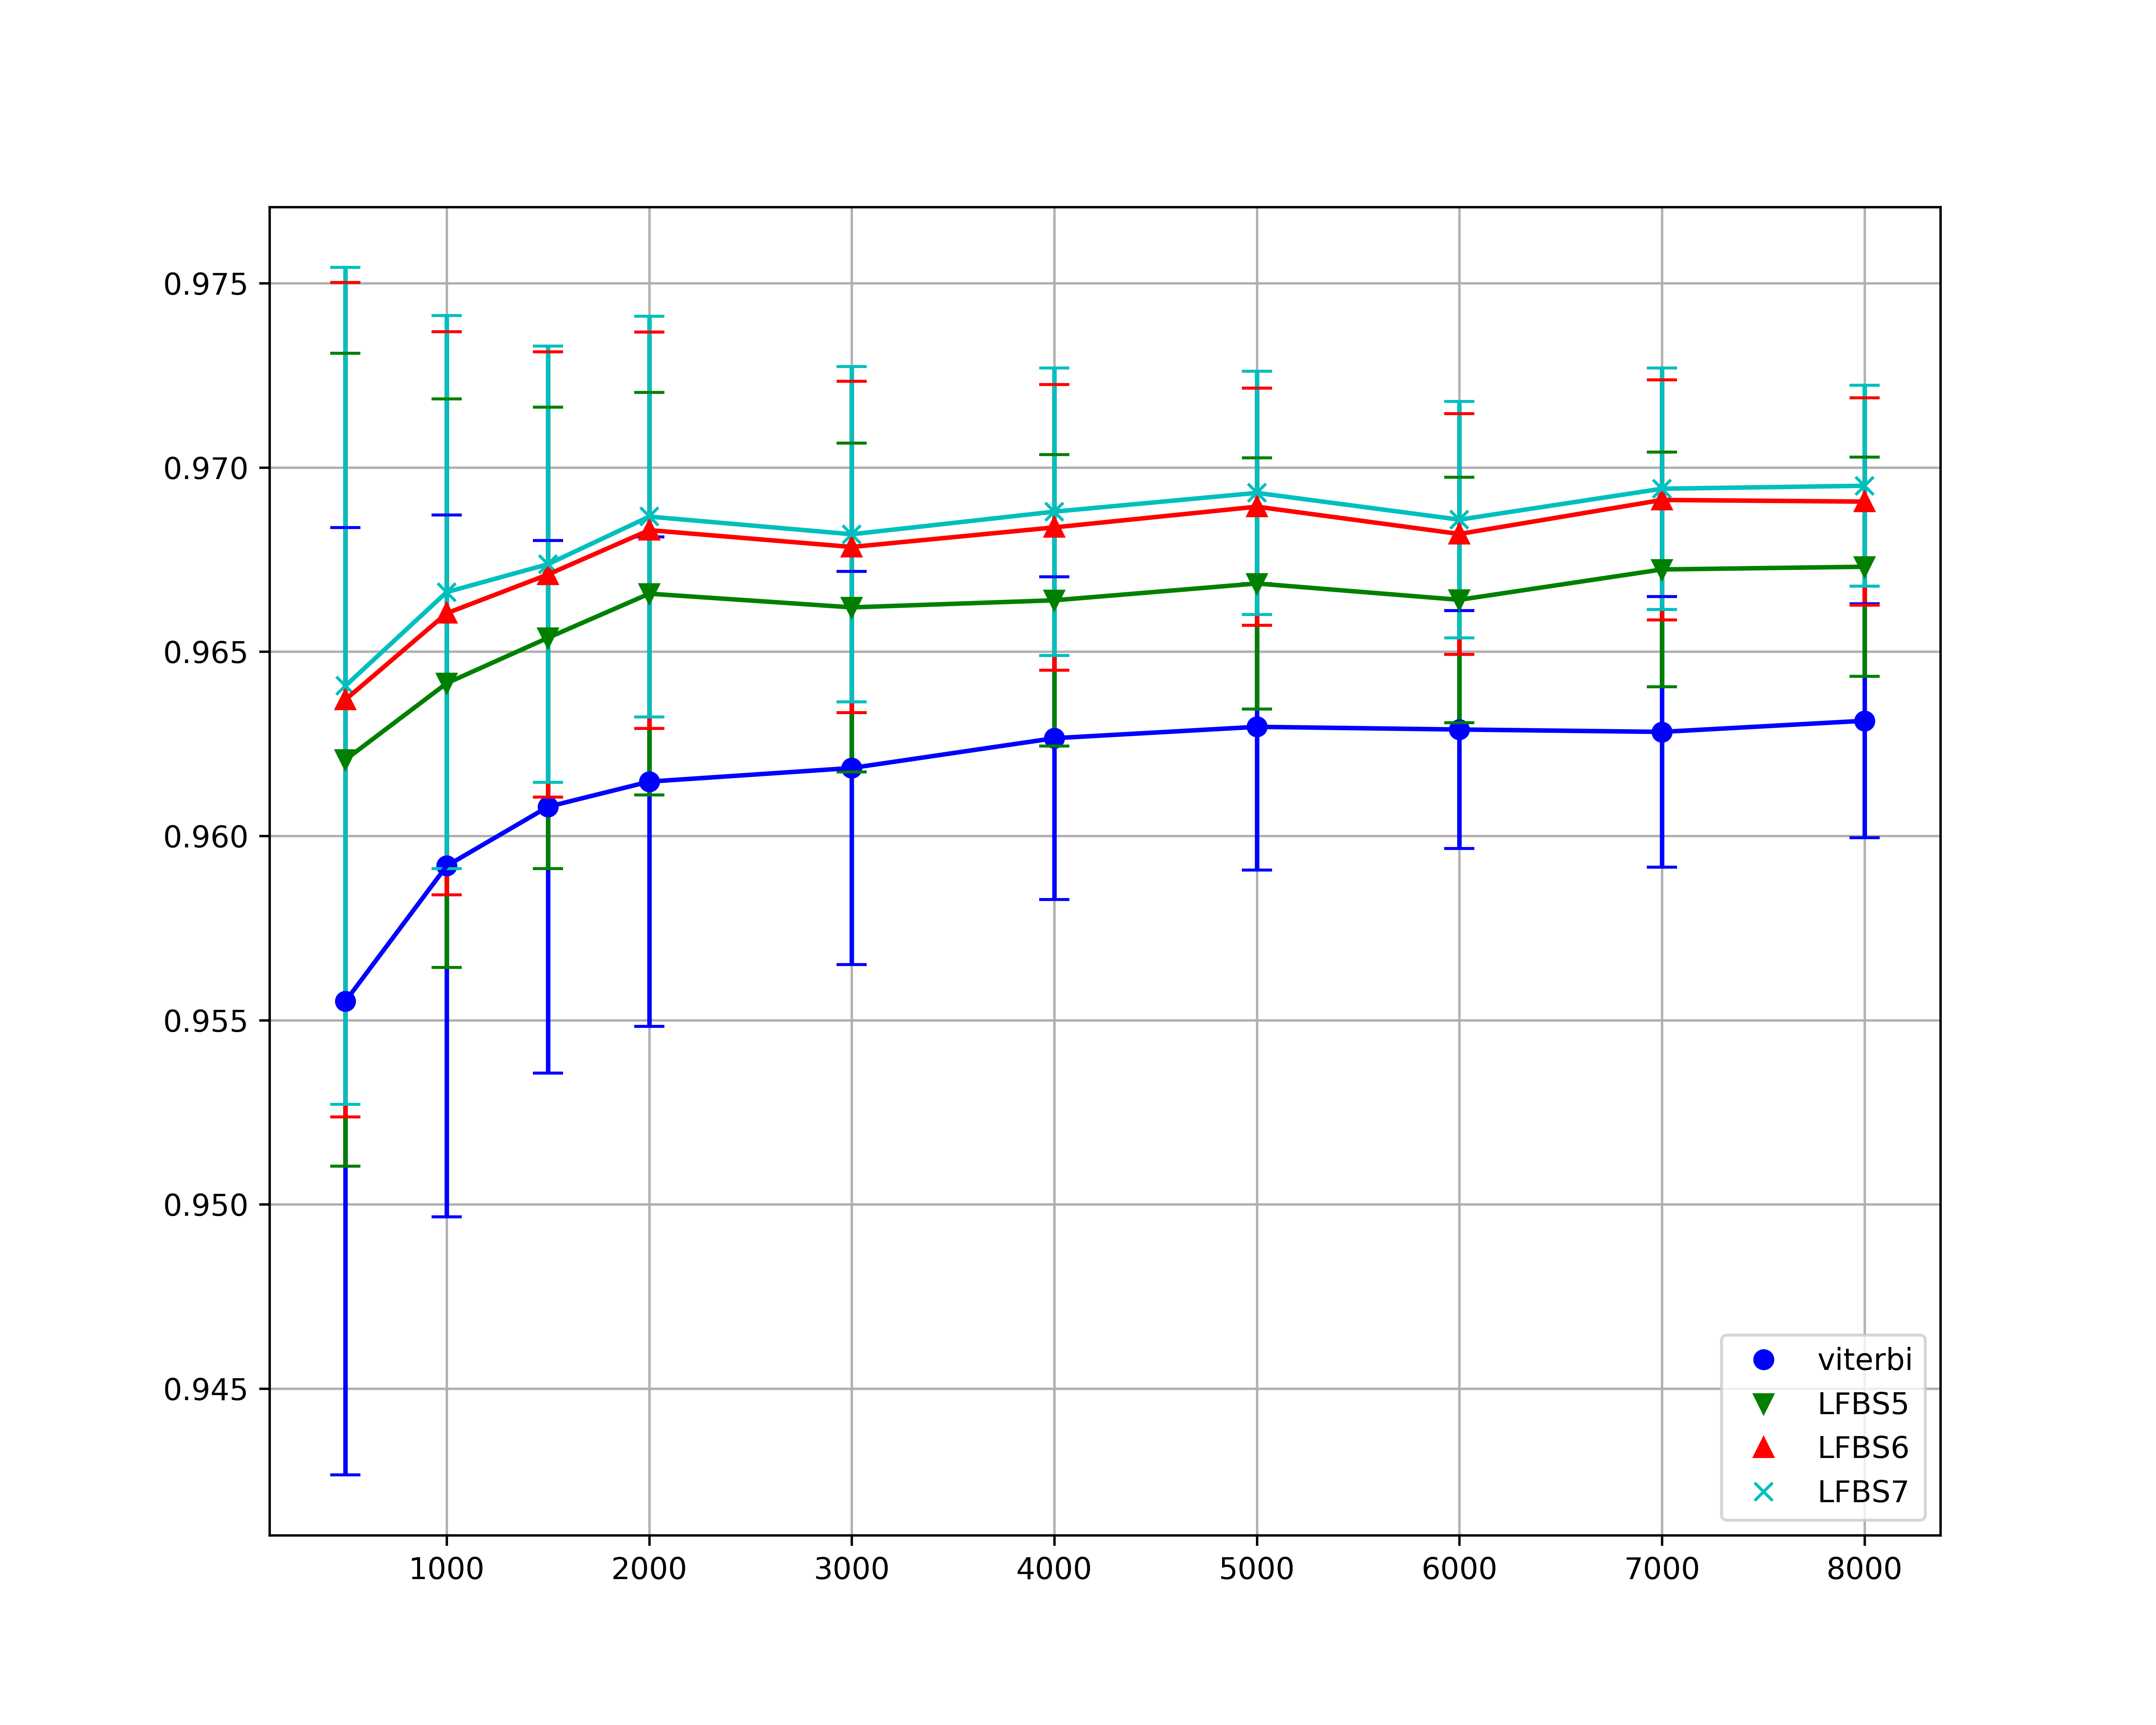}
  \caption{Sequence accuracy of the Viterbi and the LFBS algorithms with focus-length $5$, $6$ and $7$ when emission standard deviation is $2$. The mean and standard deviations are plotted against the reference length setting, with mean as marks and standard deviation as error bars.}
  \label{LFBSvar2}
\end{figure}
\begin{figure}[!htp]
  \centering
  \includegraphics[scale=0.45]{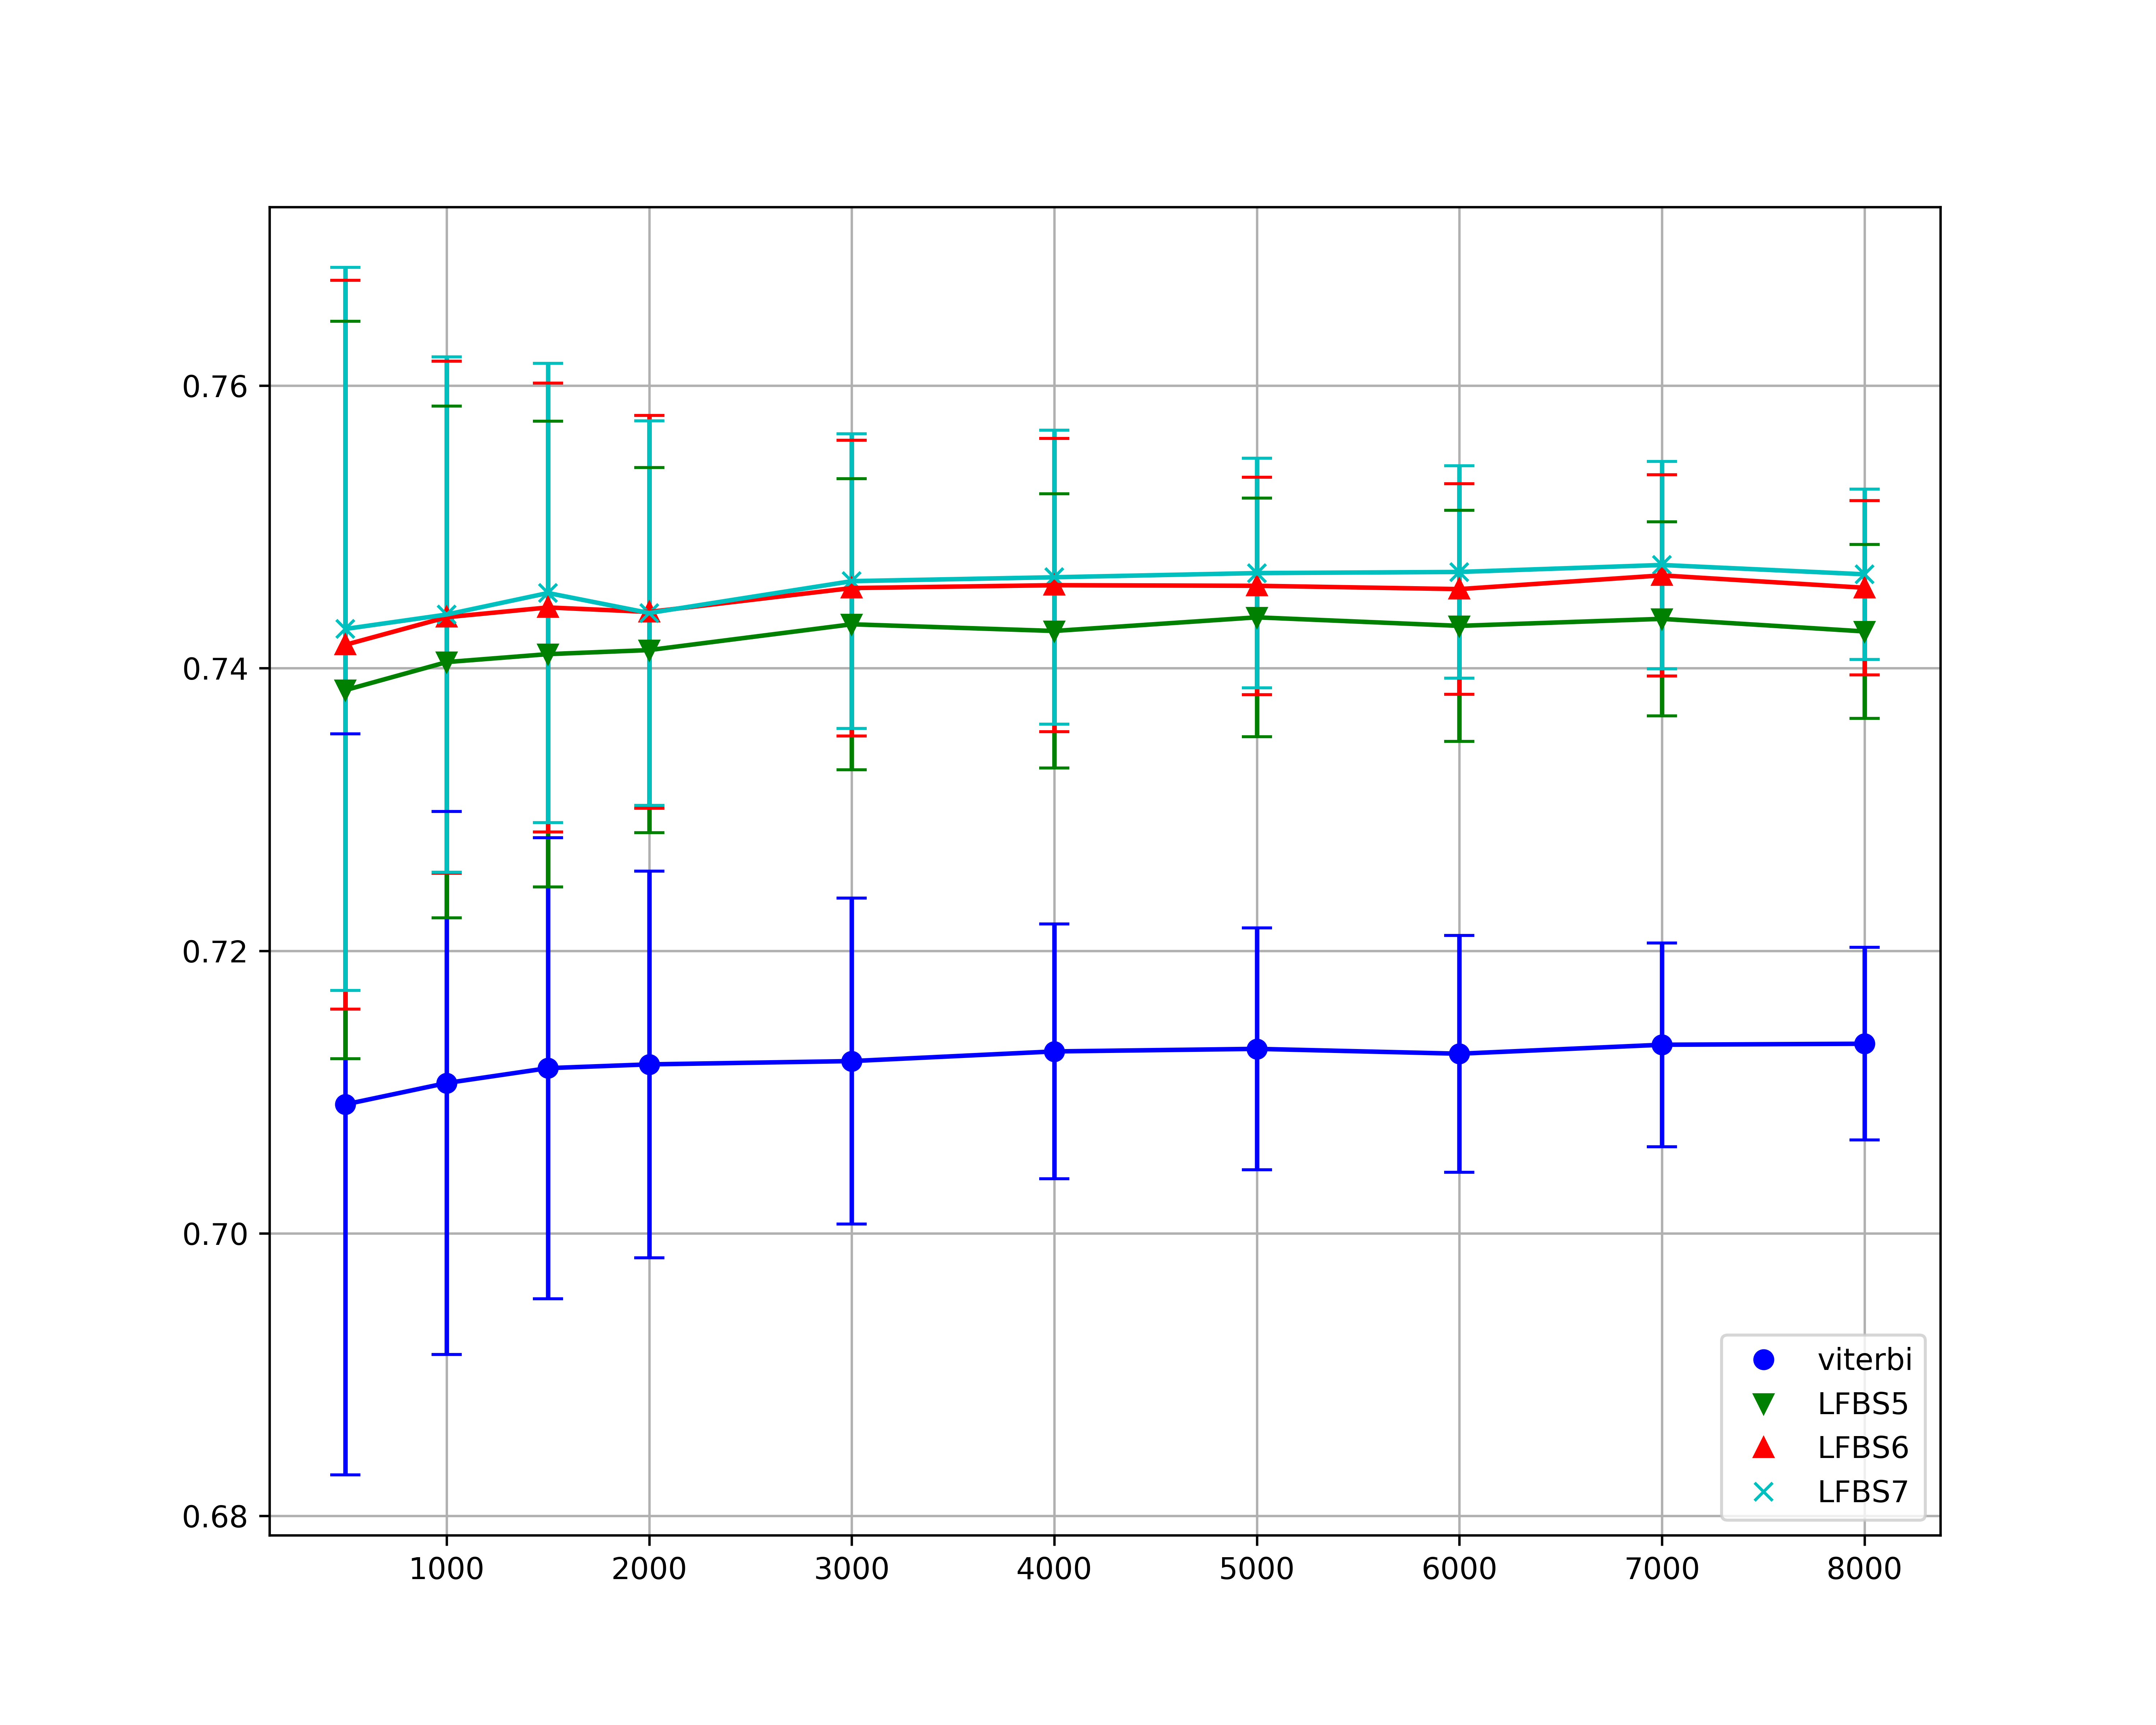}
  \caption{Sequence accuracy of the Viterbi and the LFBS algorithms with focus-length $5$, $6$ and $7$ with emission standard deviation $4$. The mean and standard deviations are plotted against the reference length setting, with mean as marks and standard deviation as error bars.}
  \label{LFBSvar4}
\end{figure}
\begin{figure}[!htp]
  \centering
  \includegraphics[scale=0.45]{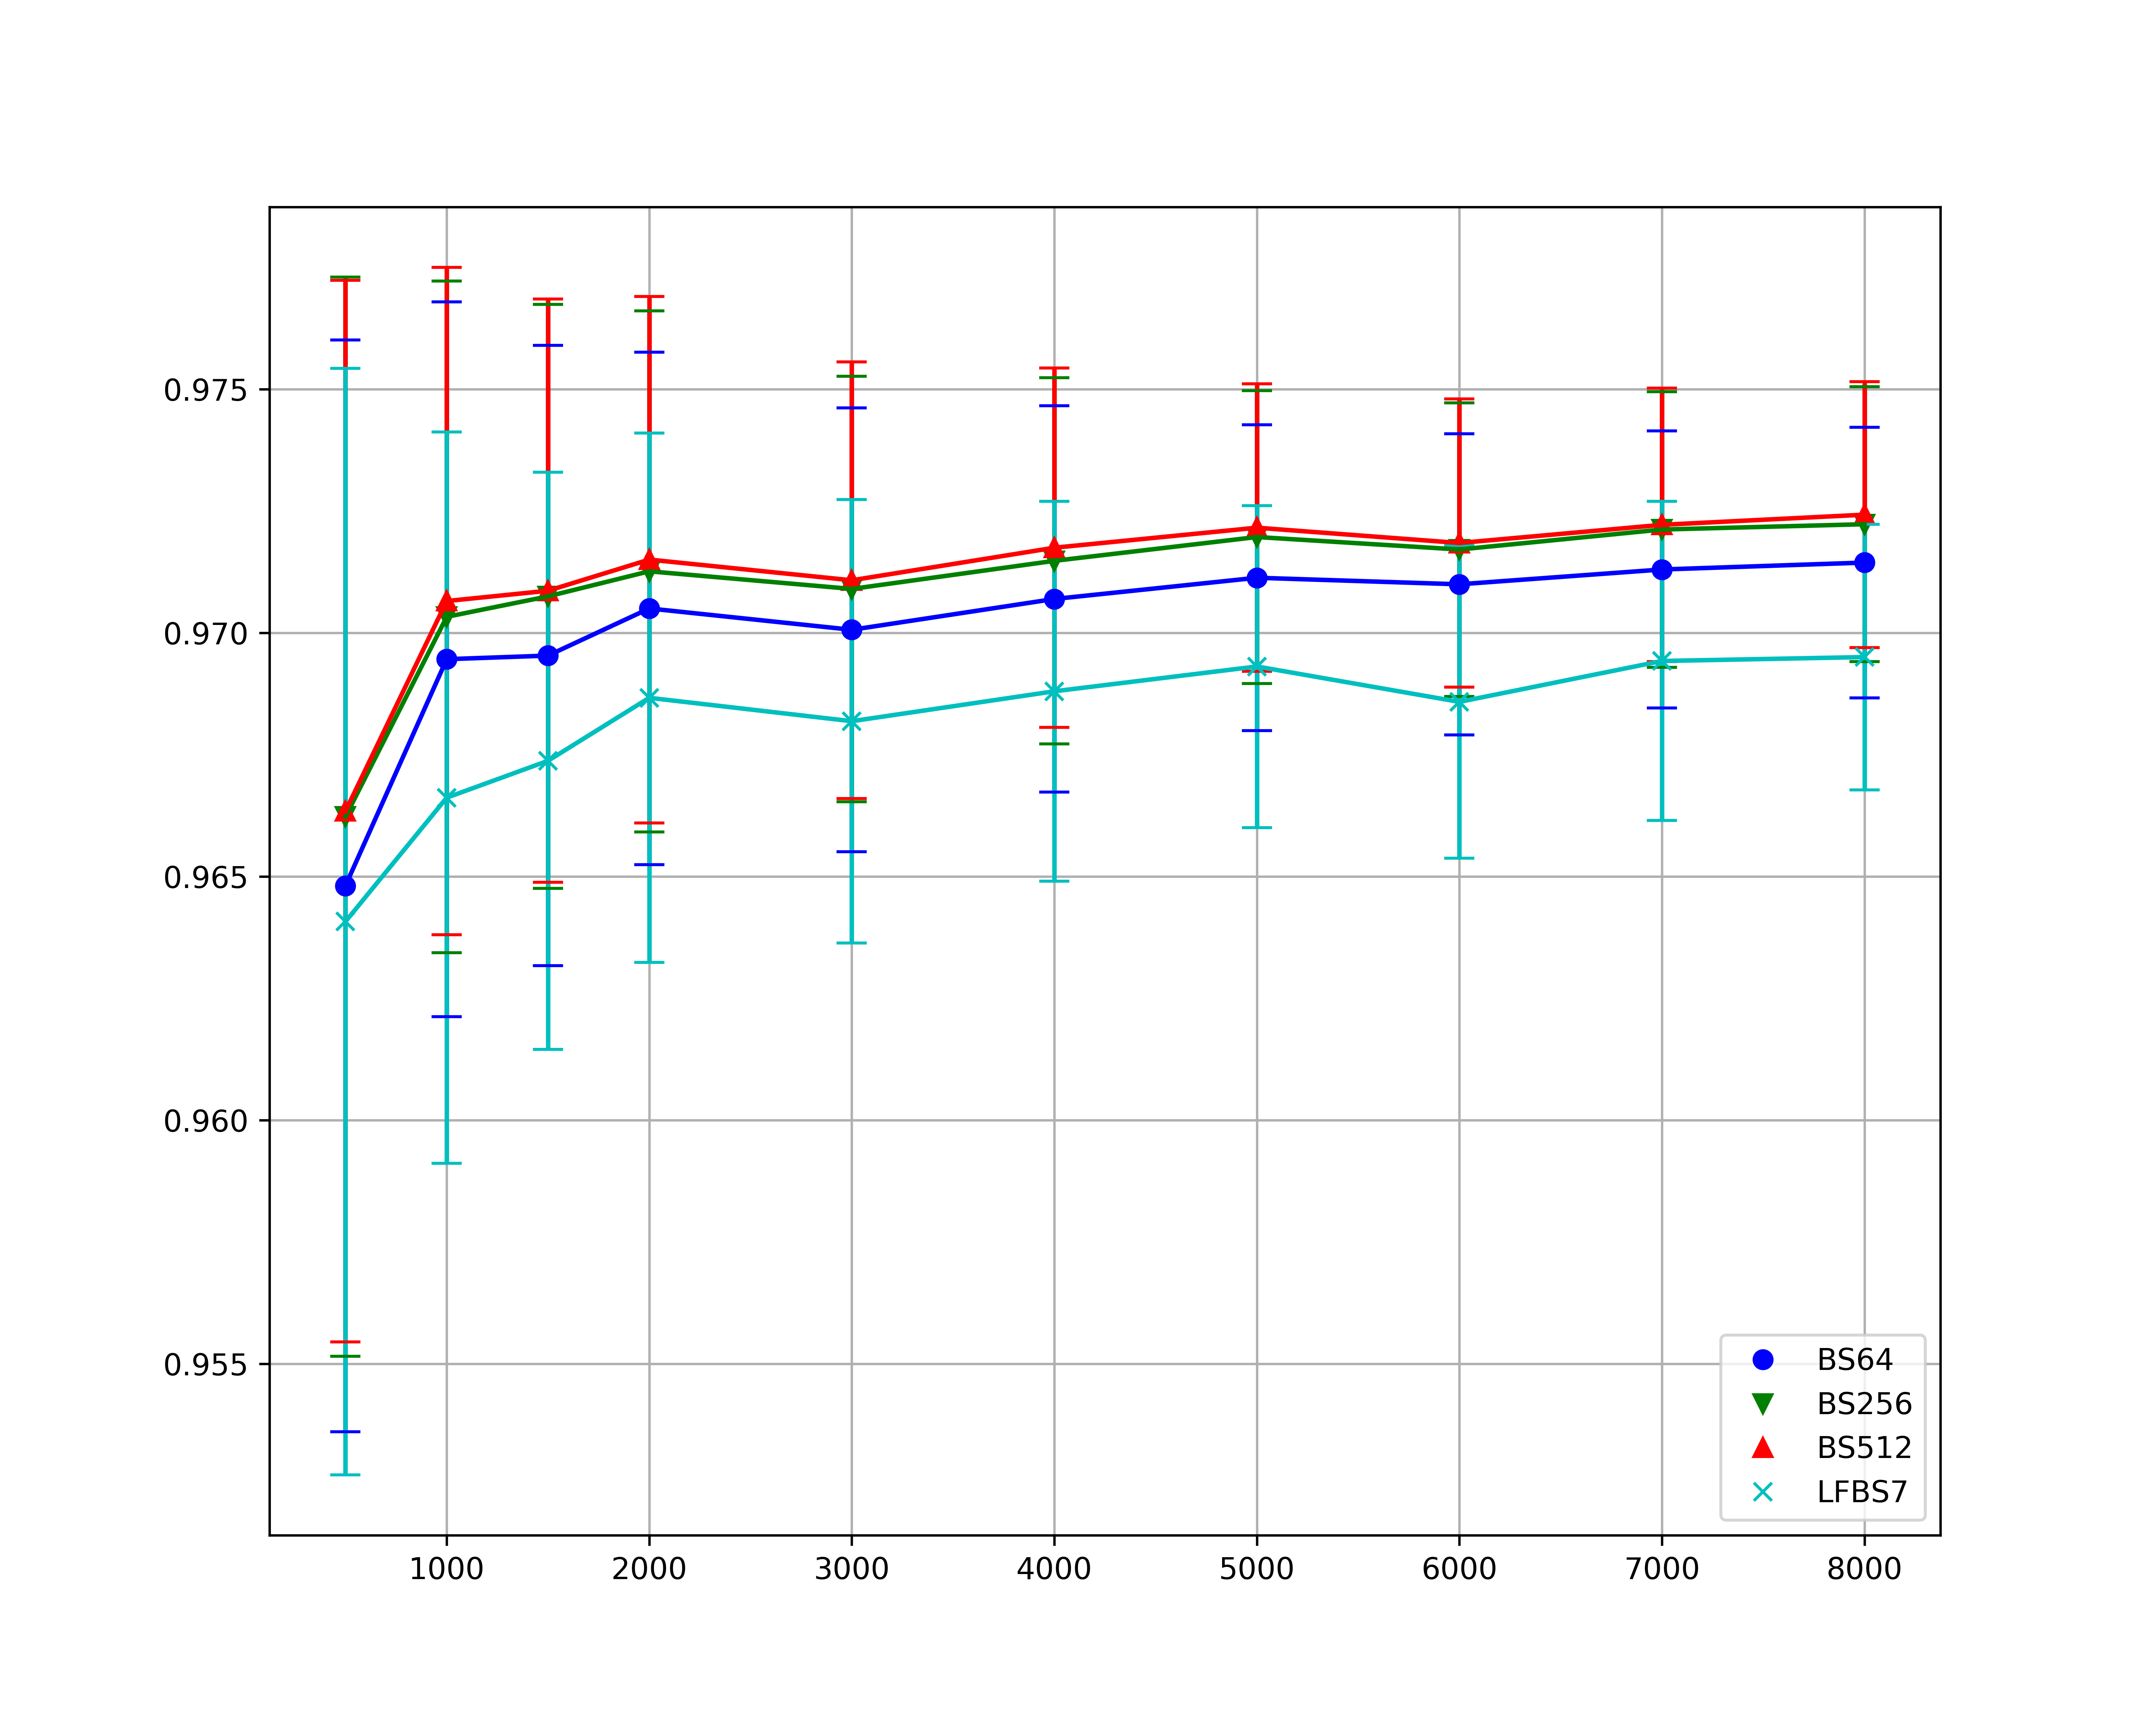}
  \caption{Sequence accuracy of the Viterbi and the GMBS algorithms with breadth-width $64$, $256$ and $512$ when emission standard deviation is $2$. The mean and standard deviations are plotted against the reference length setting, with mean as marks and standard deviation as error bars.}
  \label{BSvar2}
\end{figure} 
\begin{figure}[!hbp]
  \centering
  \includegraphics[scale=0.45]{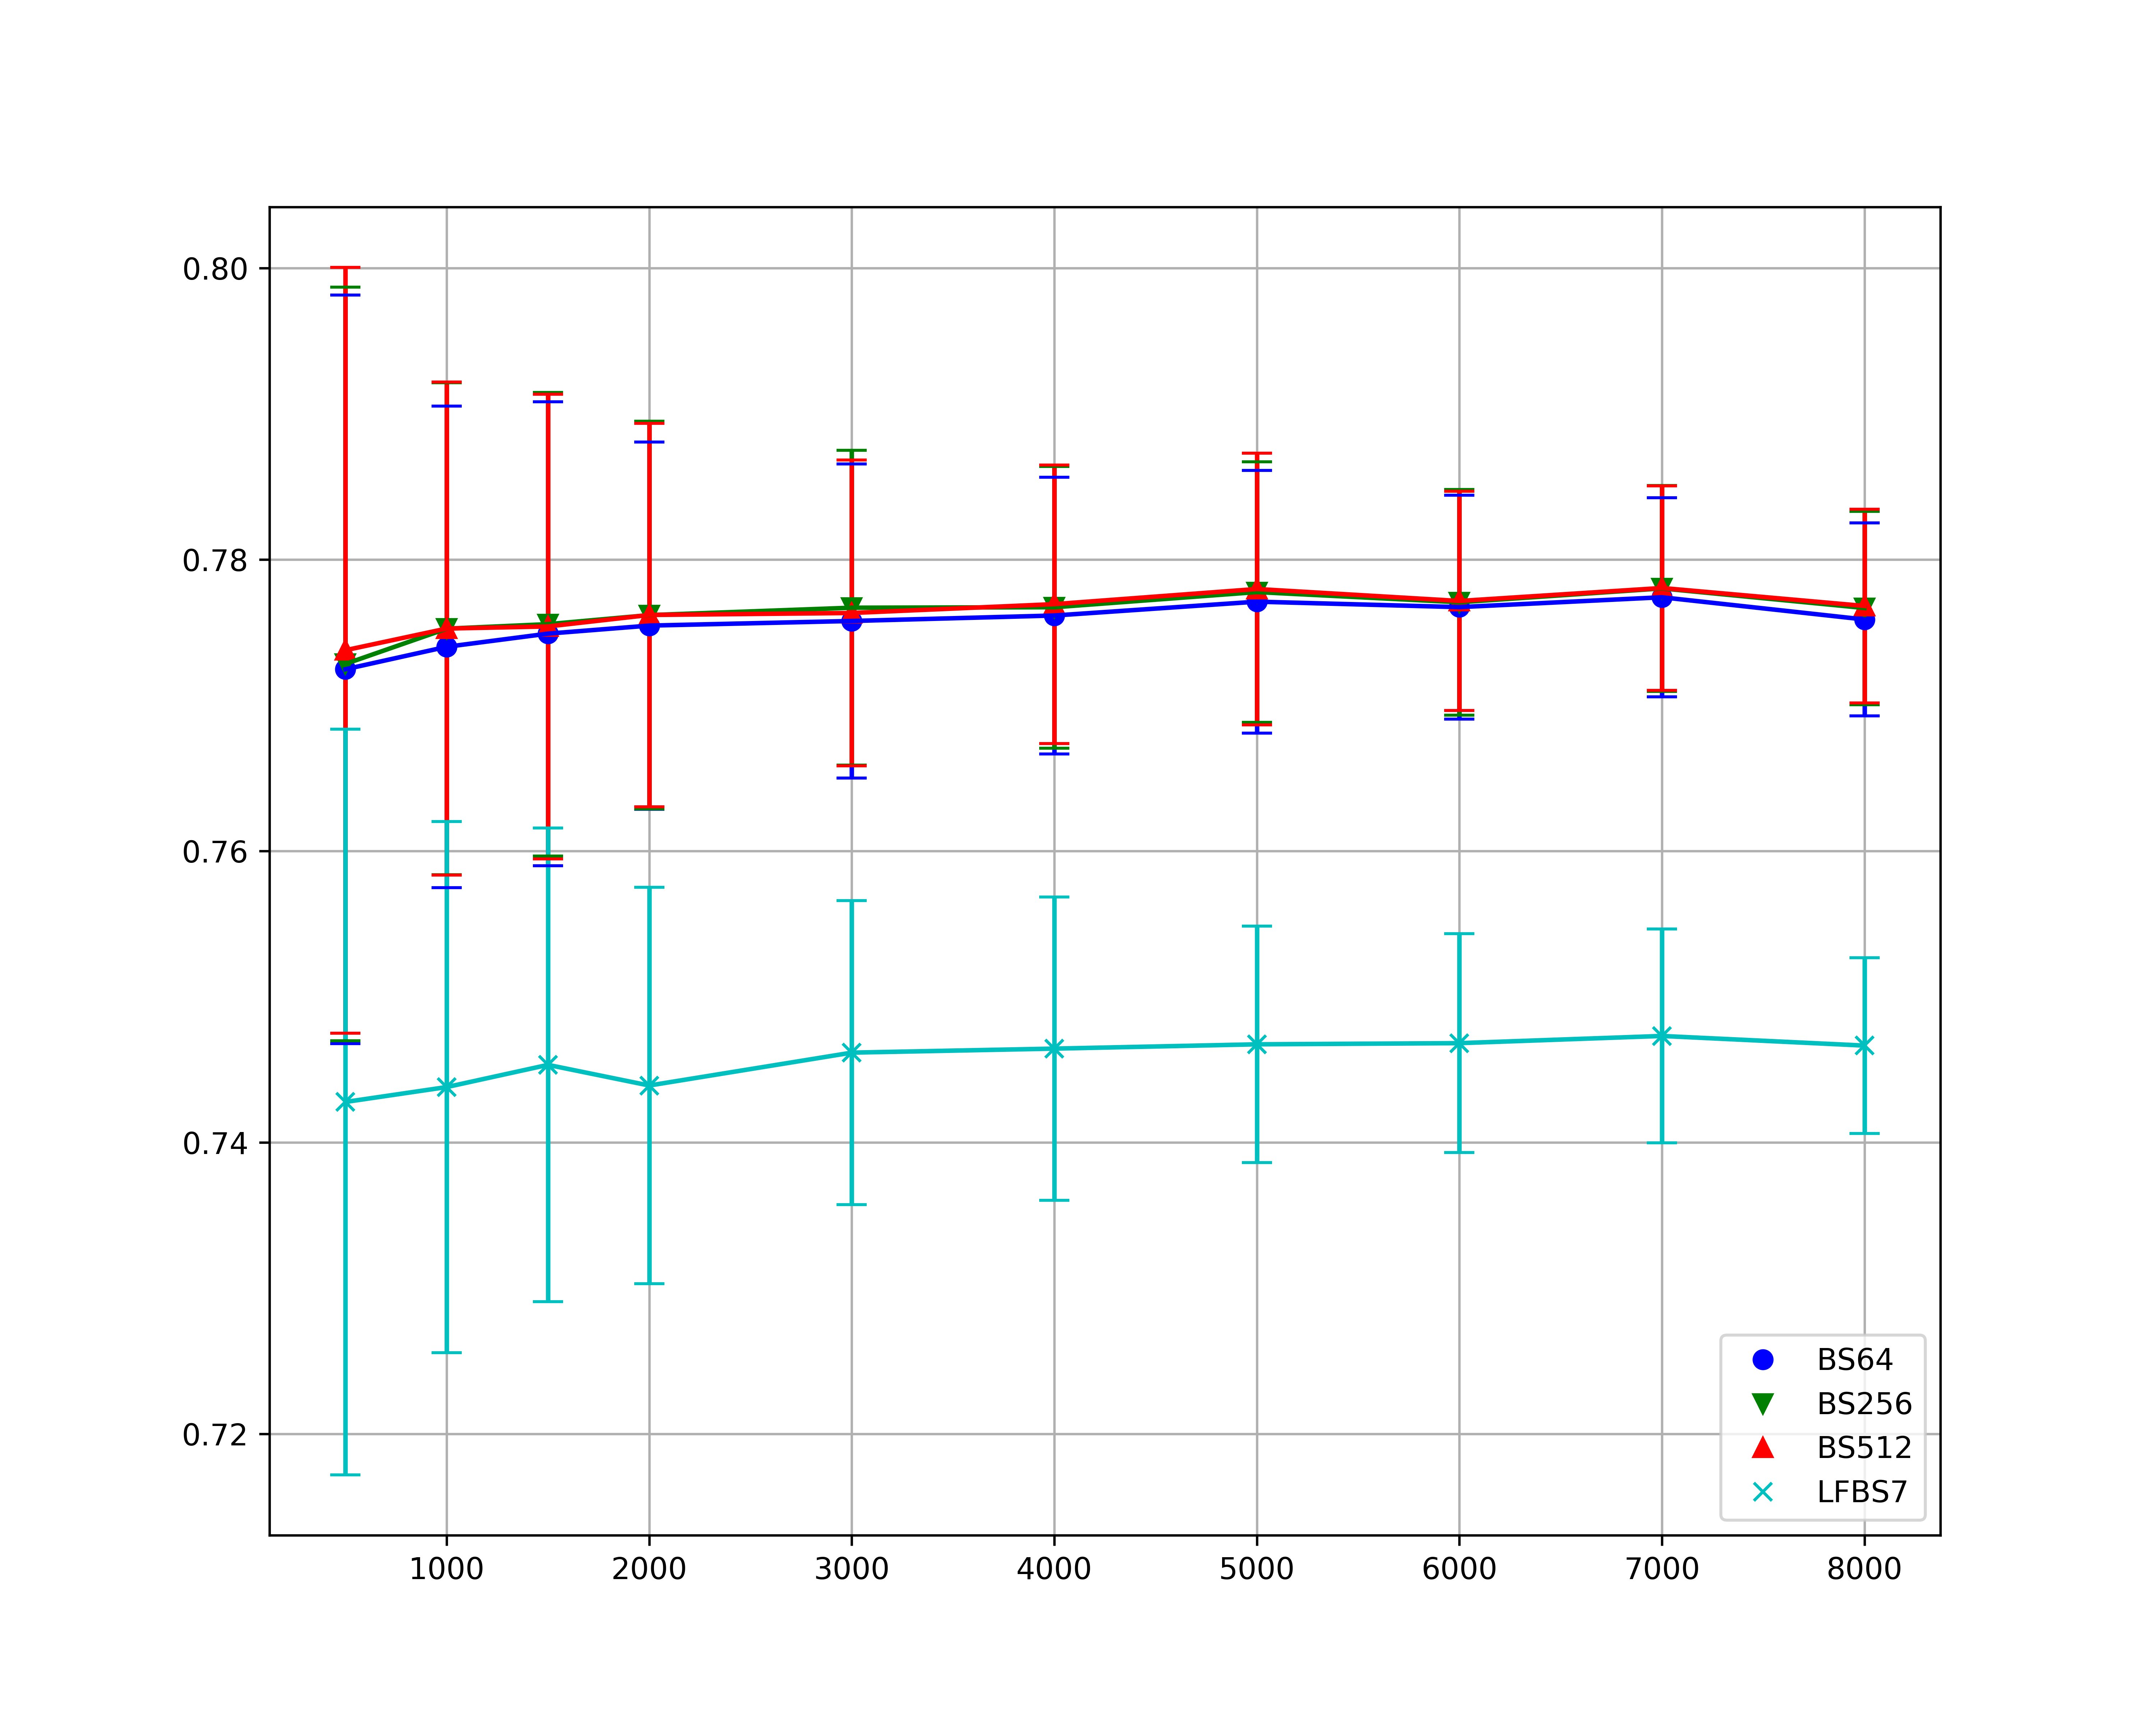}
  \caption{Sequence accuracy of the Viterbi and the GMBS algorithms with breadth-width $64$, $256$ and $512$ with emission standard deviation $4$. The mean and standard deviations are plotted against the reference length setting, with mean as marks and standard deviation as error bars.}
  \label{BSvar4}
\end{figure}
\begin{table}[!htp]\caption{Decoding performances on homopolymers with ref length $5000$ var2}\centering
\begin{tabular}{lccccccccr}
\toprule
\textbf{Methods}&\textbf{3-mer HP} &\textbf{4-mer HP} &\textbf{5-mer HP} &\textbf{6-mer HP} &\textbf{7-mer HP} &\textbf{8-mer HP}&\textbf{9-mer HP}&\textbf{10-mer HP}&Accuracy \\\hline
GMBS(8)  &$33146/35087$ & $8424/9058$ & $2763/3060$ & $618/823$ & $155/206$ & $44/67$ & $10/17$ & $1/1$ & $0.9346$\\
GMBS(64) &$33613/35175$ & $8533/9075$ & $2802/3070$ & $623/821$ & $159/208$ & $43/67$ & $10/17$ & $1/1$ & $0.9453$\\
GMBS(256)&$33657/35175$ & $8547/9077$ & $2803/3068$ & $625/821$ & $161/208$ & $43/67$ & $10/17$ & $1/1$ & $0.9466$\\
GMBS(512)&$33673/35180$ & $8543/9077$ & $2804/3069$ & $625/821$ & $160/208$ & $43/67$ & $10/17$ & $1/1$ & $0.9467$\\
LFBS(5)  &$33734/35185$ & $8607/9087$ & $2785/3069$ & $0/815$ & $0/213$ & $0/67$ & $0/16$ & $0/2$ & $0.9313$\\
LFBS(6)  &$33795/35178$ & $8628/9091$ & $2777/3067$ & $616/817$ & $0/212$ & $0/67$ & $0/16$ & $0/2$ & $0.9456$\\
LFBS(7)  &$33818/35186$ & $8629/9090$ & $2781/3067$ & $621/816$ & $153/212$ & $0/67$ & $0/16$ & $0/2$ & $0.9494$\\
Viterbi  &$32626/35244$ & $8414/9112$ & $2625/3085$ & $469/821$ & $102/212$ & $19/67$ & $3/16$ & $0/2$ & $0.9114$\\ \toprule
\end{tabular}\\{*Results are displayed as numbers of `correctly-decoded/total homopolymers'.}
\label{homo1}
\end{table}

\begin{table}[!htp]\caption{Decoding performances on homopolymers with ref length $5000$ var 4}\centering
\begin{tabular}{lcccccccccr}
\toprule
\textbf{Methods}&\textbf{3-mer HP} &\textbf{4-mer HP} &\textbf{5-mer HP} &\textbf{6-mer HP} &\textbf{7-mer HP} &\textbf{8-mer HP}&\textbf{9-mer HP}&\textbf{10-mer HP}&\textbf{11-mer HP}&Accuracy \\\hline
GMBS(8)  &$22840/34411$ & $5896/9029$ & $2088/3058$ & $474/786$ & $110/181$ & $24/54$ & $10/18$ & $1/3$ & $1/2$ & $0.6614$\\
GMBS(64) &$23694/34398$&$6021/8995$&$2209/3073$&$494/788$&$113/183$&$29/56$&$10/17$&$1/3$&$1/2$&$0.6855$\\
GMBS(256)&$23765/34379$&$6043/8971$&$2222/3075$&$500/796$&$114/180$&$28/55$&$9/17$&$2/4$&$1/2$&$0.6884$\\
GMBS(512)&$23752/34366$&$6049/8980$&$2215/3072$&$504/797$&$115/180$&$28/54$&$9/17$&$2/4$&$1/2$&$0.6883$\\
LFBS(5)  &$23589/34395$&$6168/9025$&$2029/3090$&$0/778$&$0/176$&$0/56$&$0/17$&$0/4$&$0/2$&$0.6686$\\
LFBS(6)  &$23896/34405$&$6247/9020$&$2083/3067$&$444/799$&$0/175$&$0/57$&$0/17$&$0/4$&$0/2$&$0.6871$\\
LFBS(7)  &$23995/34396$&$6308/9027$&$2130/3067$&$470/792$&$99/177$&$0/57$&$0/17$&$0/4$&$0/2$&$0.6942$\\
Viterbi  &$20882/34395$&$5677/9081$&$1888/3090$&$362/791$&$60/177$&$12/56$&$3/16$&$2/4$&$0/2$&$0.6067$\\ \toprule
\end{tabular}\\{*Results are displayed as numbers of `correctly-decoded/total homopolymers'.}
\label{homo1}
\end{table}

\begin{table}[!htp]\caption{Decoding performances lokatt and bonito}\centering
\begin{tabular}{lcccccccccr}
\toprule
\textbf{Methods}&\textbf{3-mer HP} &\textbf{4-mer HP} &\textbf{5-mer HP} &\textbf{6-mer HP} &\textbf{7-mer HP} &\textbf{8-mer HP}&\textbf{9-mer HP}&\textbf{10-mer HP}&\textbf{11-mer HP}&Accuracy \\\hline
lokatt &$984419/1214010$&$220879/319805$&$45765/103220$&$1680/30429$&$0/7311$&$0/1586$&$0/159$&$0.7472$\\
bonito_local &$919938/1129162$&$216757/297630$&$55800/96216$&$8922/28650$&$1449/6822$&$119/1509$&$2/156$&$0.7711$\\
bonito_default &$1047132/1186135$&$264549/312422$&$79075/100930$&$20500/29863$&$4202/7175$&$591/1562$&$45/168$&$0.8644$\\
\toprule
\end{tabular}\\{*Results are displayed as numbers of `correctly-decoded/total homopolymers'.}
\label{homo1}
\end{table}

\newpage
\section*{Appendix B}
The CTC graph uses a blank state to explicitly mark the ending of the previous non-blank state, hence all consecutive identical time-aligned states are considered as one sequence-aligned state. To reflect this transition construction, the marginalized BS algorithms assign a new ID to the vanilla leaf beams only if they are sourced from extending a new non-blank state after the ending of a blank state. 
\begin{figure}
  \centering
  \includegraphics[scale=0.5]{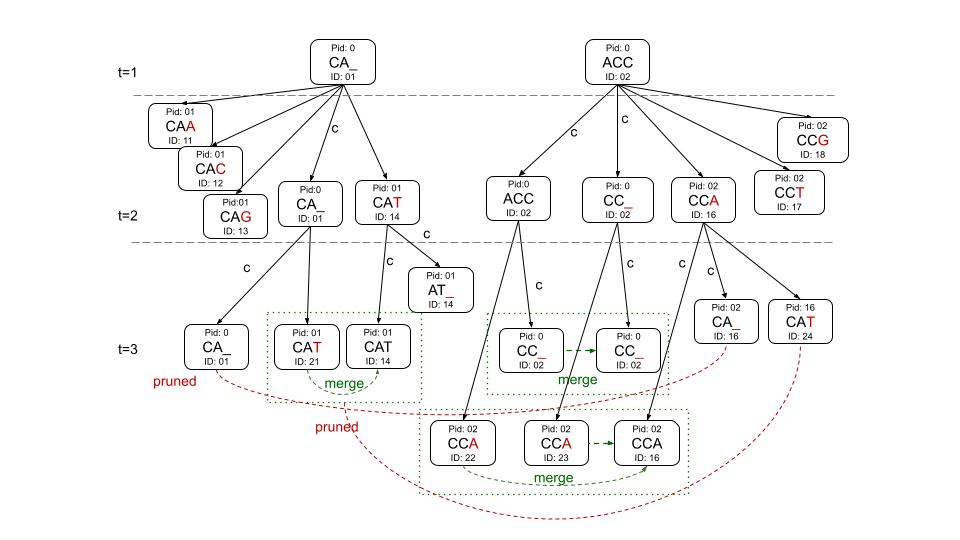}
  \caption{An implementation of the LFBS with $K=3$ on a CTC graph \cite{CTC}, given the target sequence $\{\A,\C,\C,\A\}$. The inner states transitions and leaf beams with low scores are omitted in this illustration for simplicity. Only at $t=1$ all vanilla leaf beams are listed. At $t=2$, three groups of redundant vanilla leaf beams are merged. The leaf beams with ID $21$ (representing $\{\C,\C,\A\}$) and ID $14$ (representing $\{\A,\C,\C,\A\}$) both represent the last $3$ outer states $\{\C,\C,\A\}$. The LFBS prunes the leaf beam with ID $00$ (assuming a lower score) and keeps the leaf beam with ID $14$. At $t=2$, the redundant leaf beams ID $14$ and ID $21$ (representing $\{\A,\C,\C,\A\}$) are detected and merged. In the following pruning step, the leaf beam with ID $20$ is kept while the leaf beam with ID $13$ is pruned. At $t=3$, leaf beams with ID $30$ and ID $20$ are merged (representing $\{\A,\C,\C,\A,\T\}$). In the end, the LFBS has computed $P(\{\A,\C,\C,\A,\T\},X_{1:3})$.}
  \label{LFBSDNA}
\end{figure}
